# Supplementary material for: Improving Small Molecule Generation using Mutual Information Machine
Source: arXiv:2208.09016 source file (2023-03-29)
Supplement: Supplementary file 1 [file paper-supp.tex]

%File: anonymous-submission-latex-2023.tex
\documentclass[letterpaper]{article} % DO NOT CHANGE THIS
\usepackage[submission]{aaai23}  % DO NOT CHANGE THIS
\usepackage{times}  % DO NOT CHANGE THIS
\usepackage{helvet}  % DO NOT CHANGE THIS
\usepackage{courier}  % DO NOT CHANGE THIS
\usepackage[hyphens]{url}  % DO NOT CHANGE THIS
\usepackage{graphicx} % DO NOT CHANGE THIS
\urlstyle{rm} % DO NOT CHANGE THIS
  % DO NOT CHANGE THIS
\usepackage{natbib}  % DO NOT CHANGE THIS AND DO NOT ADD ANY OPTIONS TO IT
\usepackage{caption} % DO NOT CHANGE THIS AND DO NOT ADD ANY OPTIONS TO IT
\frenchspacing  % DO NOT CHANGE THIS
\setlength{\pdfpagewidth}{8.5in} % DO NOT CHANGE THIS
\setlength{\pdfpageheight}{11in} % DO NOT CHANGE THIS
%
% These are recommended to typeset algorithms but not required. See the subsubsection on algorithms. Remove them if you don't have algorithms in your paper.
\usepackage{algorithm}
\usepackage{algorithmic}

%
% These are are recommended to typeset listings but not required. See the subsubsection on listing. Remove this block if you don't have listings in your paper.
\usepackage{newfloat}
\usepackage{listings}
\DeclareCaptionStyle{ruled}{labelfont=normalfont,labelsep=colon,strut=off} % DO NOT CHANGE THIS
\lstset{%
	basicstyle={\footnotesize\ttfamily},% footnotesize acceptable for monospace
	numbers=left,numberstyle=\footnotesize,xleftmargin=2em,% show line numbers, remove this entire line if you don't want the numbers.
	aboveskip=0pt,belowskip=0pt,%
	showstringspaces=false,tabsize=2,breaklines=true}
\floatstyle{ruled}
\newfloat{listing}{tb}{lst}{}
\floatname{listing}{Listing}
%
% Keep the \pdfinfo as shown here. There's no need
% for you to add the /Title and /Author tags.
\pdfinfo{
/TemplateVersion (2023.1)
}

\setcounter{secnumdepth}{2} %May be changed to 1 or 2 if section numbers are desired.

% The file aaai23.sty is the style file for AAAI Press
% proceedings, working notes, and technical reports.
%

\input{preamble}

% COMMENT BEFORE SUBMISSION vvvvv
\usepackage{lineno}
\linenumbers
% % COMMENT BEFORE SUBMISSION ^^^^^

% % Title

% Your title must be in mixed case, not sentence case.
% That means all verbs (including short verbs like be, is, using,and go),
% nouns, adverbs, adjectives should be capitalized, including both words in hyphenated terms, while
% articles, conjunctions, and prepositions are lower case unless they
% directly follow a colon or long dash
\title{Improving Small Molecule Generation using Mutual Information Machine - Supplementary Material}

\author {
    % Authors
    Danny Reidenbach\textsuperscript{\rm 1}\textsuperscript{\rm 2}\textsuperscript{\textasteriskcentered},%\textsuperscript{\textasteriskcentered},
    ~Micha Livne\textsuperscript{\rm 1}\textsuperscript{\textasteriskcentered}, 
    ~Rajesh K. Ilango\textsuperscript{\rm 1}, 
    ~Michelle Gill\textsuperscript{\rm 1}, 
    ~Johnny Israeli\textsuperscript{\rm 1}
}
\affiliations {
    % Affiliations
    \textsuperscript{\textasteriskcentered} equal contributions,
    % \textsuperscript{\textasteriskcentered} research was done during internship in NVIDIA\\
    \textsuperscript{\rm 1} NVIDIA, \textsuperscript{\rm 2} UC Berkeley\\
    dreidenbach@berkeley.edu, mlivne@nvidia.com, rilango@nvidia.com, mgill@nvidia.com, jisraeli@nvidia.com
}

\begin{document}

\maketitle

\appendix
\clearpage
\input{sections/supp-mat}

\bibliography{paper}

\end{document}
